# Supplementary material for: Recurrent scattering and memory effect at the Anderson localization transition
Source: arXiv:1306.2762 source file (2014-01-29)
Supplement: Supplementary file 1 [file supplementary_material_Aubry_PRL_2014.pdf]

# Supplementary material: Recurrent scattering and memory effect at the Anderson localization transition

A. Aubry,[1] L. A. Cobus,[2] S. E. Skipetrov,[3] B. A. van Tiggelen,[3] A. Derode,[1] and J. H. Page[2]

[1]*Institut Langevin, ESPCI ParisTech, CNRS UMR 7587, Université Denis Diderot - Paris 7, 1 rue Jussieu, 75005 Paris, France*

[2]*Department of Physics and Astronomy, University of Manitoba, Winnipeg, Manitoba R3T 2N2, Canada*

[3]*Université Grenoble 1/CNRS, Laboratoire de Physique et Modélisation des Milieux Condensés UMR 5493, B.P. 166, 38042 Grenoble, France*

## RECURRENT SCATTERING FILTER

This section describes the method to separate the recurrent scattering (RS) and the conventional multiple scattering (MS) contributions. Our approach is inspired by previous studies that have shown how to separate single scattering (SS) and MS in weakly scattering media [S1–S3]. RS actually displays the same statistical properties as SS, *i.e* a deterministic spatial coherence along the antidiagonals of the array reponse matrix $\mathbf{K}$, which is a manifestation of a long-range memory effect. The idea is to take advantage of this property to filter RS from the conventional MS background. However, albeit more restricted, a memory effect also exists for the MS contribution [S4, S5]. For the matrix $\mathbf{K}$, this implies that the MS far-field speckle exhibits a finite correlation length $\delta$ [S6, S7], which can be expressed in units of the array pitch $p$ as

$$\delta \sim \lambda_w a/[pW(t)], \tag{S1}$$

with $\lambda_w$ the wavelength in water, $a$ the array-sample distance and $W(t)$ the dynamic size of the diffusive halo as a function of time. In a weakly scattering regime, the diffusive halo grows quickly enough ($W(t) \propto \sqrt{Dt}$, with $D$ the diffusion constant) to consider the multiple scattering field as fully uncorrelated. The separation of SS and MS is then relatively easy [S1–S3]. In a strongly scattering regime, the diffusive halo grows much more slowly and can even saturate at the Anderson transition. Hence, the separation between RS and conventional MS is more tricky but still possible.

The method used for this separation consists of a four-step process:

• Rotation of the matrix $\mathbf{K}(t)$ and construction of two submatrices $\mathbf{A^{(1)}}(t)$ and $\mathbf{A^{(2)}}(t)$.

• Singular value decomposition (SVD) of matrices $\mathbf{A^{(q)}}$ (with $q = 1, 2$) in the frequency domain. $\mathbf{A^{(q)}}$ is decomposed as the sum of two matrices: $\mathbf{A^{(q)}} = \mathbf{S} + \mathbf{N}$, where $\mathbf{S}$ and $\mathbf{N}$ correspond to the signal subspace mainly associated with RS and the noise subspace associated with conventional MS.

• Correction of the signal and noise subspaces to obtain estimators of the RS and MS contributions in the time domain: $\hat{\mathbf{A}}^{(\mathbf{q})}_{\mathbf{R}}(t)$ and $\hat{\mathbf{A}}^{(\mathbf{q})}_{\mathbf{M}}(t)$. This correction is based on energy arguments.

• Construction from $\hat{\mathbf{A}}^{(\mathbf{q})}_{\mathbf{R}}(t)$ and $\hat{\mathbf{A}}^{(\mathbf{q})}_{\mathbf{M}}(t)$ of RS and MS matrix estimators $\hat{\mathbf{K}}_{\mathbf{R}}(t)$ and $\hat{\mathbf{K}}_{\mathbf{M}}(t)$.

The first, second and fourth steps (rotation of data, SVD of antidiagonals) have already been presented in a previous study [S3] and will be briefly recalled. The third step constitutes the important new extension of the previous method. This novel step is necessary to tackle the medium-range correlations of the MS field in the strongly scattering regime.

### Matrix rotation

A rotation of matrix data is performed as depicted in Fig. S1(a)-(b). It consists in building two matrices $\mathbf{A^{(1)}}$ and $\mathbf{A^{(2)}}$ from matrix $\mathbf{K}$:

$$\mathbf{A^{(1)}} = \left[A^{(1)}_{lm}\right] \text{ of dimension } (2M-1)\times(2M-1),$$
$$\text{such that } A^{(1)}[l,m] = K[l+m-1, m-l+2M-1] \tag{S2}$$
$$\mathbf{A^{(2)}} = \left[A^{(2)}_{lm}\right] \text{ of dimension } (2M-2)\times(2M-2),$$
$$\text{such that } A^{(2)}[l,m] = K[l+m, m-l+2M-1] \tag{S3}$$

with $M = (N+3)/4$. Here $N = 61$, so $M = 16$ is an even number. This rotation of data is illustrated in Fig. S1. Fig. S1(a) shows an example of matrix $\mathbf{K}$ measured experimentally at a given time $t$. Fig. S1(b) displays the matrix $\mathbf{A^{(1)}}$ obtained after the rotation of data described above. The columns of matrices $\mathbf{A^{(1)}}$ and $\mathbf{A^{(2)}}$ correspond to the antidiagonals of $\mathbf{K}$. Therefore the coherence of recurrent scattering now manifests itself along the columns of $\mathbf{A^{(1)}}$ and $\mathbf{A^{(2)}}$. $\mathbf{A^{(1)}}$ contains the antidiagonals for which the source index $s$ and the receiver index $r$ are of same parity, such that $l = (s-r)/2 + M + 1$ and $m = (s+r)/2 - M + 1$ are integers. $\mathbf{A^{(2)}}$ contains the antidiagonals for which $s$ and $r$ are of opposite parity, such that $l = (s-r-1)/2 + M$ and $m = (s+r+1)/2 + M$ are integers. In the next subsection, we will no longer make the difference between matrices $\mathbf{A^{(1)}}$ and $\mathbf{A^{(2)}}$ because they are filtered in the same way. They will both be called $\mathbf{A}$. $P$ is the dimension of $\mathbf{A}$. For matrix $\mathbf{A^{(1)}}$, $P = 2M - 1$; for matrix $\mathbf{A^{(2)}}$, $P = 2M - 2$. Because of spatial reciprocity, $\mathbf{K}$ is symmetric ($k_{sr} = k_{rs}$). Thus, $\mathbf{A}$ also exhibits a symmetry: each line of its upper part is identical to a line of its lower part.

### Singular value decomposition of A

A Fourier analysis of the matrix $\mathbf{A}(t)$ is first performed by means of a discrete Fourier transform (DFT). This yields a set

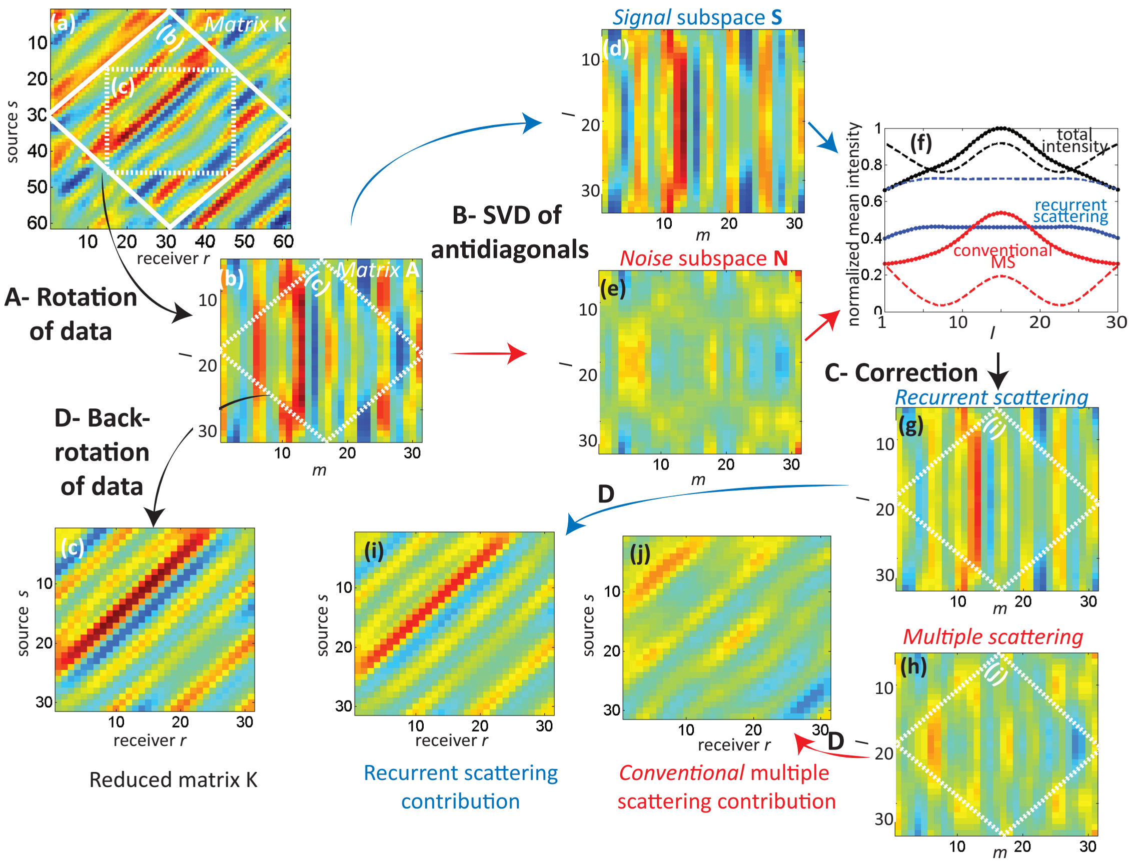


FIG. S1: Different steps for the separation of RS and MS illustrated for a representative example of the matrix $\mathbf{K}$ at a given time $t = 185$ $\mu$s and frequency $f = 1.25$ MHz. (a) Measured matrix $\mathbf{K}$. (b) Matrix $\mathbf{A}^{(1)}$ deduced from $\mathbf{K}$ by rotation of data. (c) Reduced matrix $\mathbf{K}$ deduced from $\mathbf{A}$ by back-rotation of data. (d) Signal subspace $\mathbf{S}$ of $\mathbf{A}$ [Eq. (S9)]. (e) Noise subspace $\mathbf{N}$ of $\mathbf{A}$ [Eq. (S10)]. (f) Intensity profiles of antidiagonal matrices: total intensity $I$ (continuous black line), signal subspace intensity $I_S$ (blue dashed line), noise subspace intensity $I_N$ (red dashed line), $I_S + I_N$ (black dashed line), estimated RS intensity $\hat{I}_R$ (blue continuous line), estimated MS intensity $\hat{I}_M$ (red continuous line). (g) Estimated RS antidiagonal matrix $\hat{\mathbf{A}}_{\mathbf{R}}$. (h) Estimated MS antidiagonal matrix $\hat{\mathbf{A}}_{\mathbf{M}}$. (i) Estimated RS matrix $\hat{\mathbf{K}}_{\mathbf{R}}$. (j) Estimated MS matrix $\hat{\mathbf{K}}_{\mathbf{M}}$.

of matrices $\mathbf{A}(f)$ at each frequency $f$. The matrix $\mathbf{A}$ contain a SS/RS component (matrix $\mathbf{A}_{\mathbf{R}}$) and MS component $\mathbf{A}_{\mathbf{M}}$ that we want to separate:

$$\mathbf{A} = \mathbf{A}_{\mathbf{R}} + \mathbf{A}_{\mathbf{M}} \tag{S4}$$

Using the paraxial approximation to describe the wave propagation outside of the scattering sample and assuming point-like scatterers, the SS/RS contribution can be expressed as [S1–S3]

$$A_R[l,m] = \exp\left[j\frac{k_w p^2}{4a}(s-r)^2\right] r_m \tag{S5}$$

with $k_w$ the wave number in water and $r_m$ a random coefficient. Remember that $l = (s-r)/2 + M + 1$ for $A^{(1)}[l,m]$ and that $l = (s-r-1)/2 + M$ for $A^{(2)}[l,m]$. Hence, each column of the matrix $\mathbf{A}_{\mathbf{R}}$ exhibits a known dependence as a function of index $l$ (parabolic phase term) which is the manifestation of a long-range memory effect. On the contrary, the MS contribution does not display such a deterministic behavior. It can be expressed as a correlated random wave field:

$$A_M[l,m] = c_l d_m \tag{S6}$$

where $c_l$ and $d_m$ are random coefficients. The memory effect gives rise to a correlation between the lines of $\mathbf{A}_{\mathbf{M}}$. This correlation can be quantified with the coefficient $\Gamma[l'] =< c_l c^*_{l+l'} >$. We define the correlation length $\delta$ as the typical length scale of this correlation. In the experimental conditions of the Letter, a typical value for $\delta$ is of 4 array pitches.

As in Ref. S3, a singular value decomposition (SVD) of the matrix $\mathbf{A}$ can be performed to separate SS/RS from MS. The SVD decomposes a matrix into two subspaces: a *signal* subspace (a matrix characterized by a long-range correlation between its lines and/or columns) and a *noise* subspace (a random matrix with possibly some short or medium-range correlations between its entries). When the SVD is applied to the matrix $\mathbf{A}$, we expect the *signal* subspace (*i.e.*, the largest sin-

gular values) to correspond to the SS/RS contribution ($\mathbf{A_R}$) and the *noise* subspace (*i.e.*, the smallest singular values) to correspond to the MS contribution ($\mathbf{A_M}$).

The SVD of matrix $\mathbf{A}$ is given by

$$\mathbf{A} = \mathbf{U\Lambda V}^{\dagger} = \sum_{q=1}^{P} \lambda_q \mathbf{U^{(q)}} \mathbf{V^{(q)}}^{\dagger} \tag{S7}$$

where the symbol † stands for transpose conjugate. $\mathbf{\Lambda}$ is a square diagonal matrix of dimension $N$, containing the real positive singular values $\lambda_q$ in a decreasing order ($\lambda_1 > \lambda_2 > ... > \lambda_P$). $\mathbf{U}$ and $\mathbf{V}$ are square unitary matrices of dimension $N$. Their respective columns $\mathbf{U^{(q)}}$ and $\mathbf{V^{(q)}}$ correspond to the singular vectors associated with each singular value $\lambda_q$.

A general issue is to determine which rank of singular value separates the *signal* subspace from the *noise* subspace [S3]. However, the paraxial approximation can be made here since the array-sample distance $a$ is much larger than the tranverse size of the array $Np$. The SS/RS contribution is then given by Eq. (S5) and $\mathbf{A_R}$ is of rank 1. Hence, only the eigenspace associated with the first singular value $\lambda_1$ corresponds to the signal subspace. For point-like scatterers, the elements of $\mathbf{U^{(1)}}$ are given by

$$u_l^{(1)} = \exp\left[j\frac{k_w p^2}{4a}(s-r)^2\right] / \sqrt{P} \tag{S8}$$

with $l = (s-r)/2+M+1$ for $\mathbf{A^{(1)}}$ and $l = (s-r-1)/2+M$ for $\mathbf{A^{(2)}}$. In practice, due to the directivity of transducers and the finite size of scatterers, the modulus of $\mathbf{U^{(1)}}$ is not perfectly uniform. Consequently, a SVD of $\mathbf{A}$ is needed to estimate the SS/RS subspace with the best precision. The signal ($\mathbf{S}$) and noise ($\mathbf{N}$) subspaces are thus given by,

$$\mathbf{S} = \mathbf{U^{(1)}U^{(1)\dagger}A} \tag{S9}$$
$$\mathbf{N} = \mathbf{A} - \mathbf{U^{(1)}U^{(1)\dagger}A} \tag{S10}$$

An example of the result provided by the SVD of $\mathbf{A}$ is shown in Fig. S1. The signal and noise subspaces deduced from $\mathbf{A}$ [Fig. S1(b)] are shown in Fig. S1(d) and (e), respectively. Ideally, $\mathbf{S}$ should be devoid of conventional MS. However, the latter contribution is not strictly orthogonal to the SS/RS subspace, especially as the MS field exhibits medium-range correlations. Hence, a post-treatment is needed to correct this contamination of the signal subspace by MS.

### Correction of the signal and noise subspaces

An inverse discrete Fourier transform is first performed to return to the time domain. This yields the signal and noise subspaces as a function of time $t$, $\mathbf{S}(t)$ and $\mathbf{N}(t)$. The partial mixing of RS and MS in noise and signal subspaces can be pointed out by investigating the intensity profiles $I_S$ and $I_N$ as a function of $l$ which is directly related to the distance between the source $s$ and the receiver $r$:

$$I_S[l] = \left\langle |S_{lm}|^2 \right\rangle \text{ and } I_N[l] = \left\langle |N_{lm}|^2 \right\rangle \tag{S11}$$

where the symbol $< \cdots >$ denotes an ensemble average. We have checked that these mean intensities are indeed independent of $m$. An example of the intensity profiles obtained at a given time $t$ is shown in Fig.S1(f). Whereas the intensity profile $I_S$ associated with the signal subspace is a flat plateau characteristic of single/recurrent scattering, the intensity profile $I_N$ does not display an intensity profile typical of multiple scattering, *i.e* a coherent backscattering peak on top of a flat incoherent background. This is because a part of the MS contribution emerges along the signal subspace. One can also note that the sum of $I_S$ and $I_N$ is not equal to the total intensity $I[l] = \left\langle |A_{lm}|^2 \right\rangle$ computed from the matrix $\mathbf{A}$. Although the subspaces $\mathbf{S}$ and $\mathbf{N}$ are orthogonal in the frequency domain, they are not necessarily so in the time domain.

To investigate the coupling between RS and MS eigenspaces, $\mathbf{S}$ and $\mathbf{N}$ can be expressed as a function of $\mathbf{A_R}$ and $\mathbf{A_M}$ by substituting Eq. (S4) into Eqs. (S9) and (S10). This yields

$$\mathbf{S} = \mathbf{A_R} + \mathbf{U^{(1)}U^{(1)\dagger}A_M} \tag{S12}$$
$$\mathbf{N} = \mathbf{A_M} - \mathbf{U^{(1)}U^{(1)\dagger}A_M} \tag{S13}$$

This last pair of equations points out the coupling term $\mathbf{U^{(1)}U^{(1)\dagger}A_M}$.

We now derive the expressions of the noise and signal matrix elements $N[l,m]$ and $S[l,m]$, as well as the corresponding intensities $I_N[l]$ and $I_S[l]$. An expression for the noise matrix entries $N[l,m]$ can be found by substituting Eq. (S6) into Eq. (S13):

$$N[l,m] = \left[c_l - u_l^{(1)} \sum_{i=1}^{P} u_i^{(1)*} c_i\right] d_m \tag{S14}$$

The intensity $I_N[l]$ [Eq. (S11)] can then be deduced:

$$I_N[l] = \left[ <|c_l|^2> - 2Re\left\{ u_l^{(1)} \sum_{i=1}^{P} u_i^{(1)*}\Gamma[l-i] \right\} + \left|u_l^{(1)}\right|^2 \sum_{i=1}^{P}\sum_{j=1}^{P} u_i^{(1)*}u_j^{(1)}\Gamma[i-j] \right] <|d_m|^2> \tag{S15}$$

Making the approximation that $\Gamma[i] = 0$ for $|i| > \delta$ and assuming that $2a/k_w >> p^2\delta^2$ (valid in our experiment), then $u_i^{(1)*}u_j^{(1)} \sim 1/P$ for $|i-j| < \delta$ and the last equation becomes

$$I_N[l] = \left[ <|c_l|^2> - \frac{2}{P}\sum_{i=1}^{P}\Gamma[l-i] + \frac{1}{P^2}\sum_{i=1}^{P}\sum_{j=1}^{P}\Gamma[i-j] \right] <|d_m|^2> \tag{S16}$$

Finally, if $P >> \delta$ (which is the case in our experiment), $\sum_{i=1}^{P}\sum_{j=1}^{P}\Gamma[i-j] \sim 2P\sum_{m=0}^{\delta}\Gamma[m]$. It then follows that

$$I_N[l] = \underbrace{<|c_l|^2><|d_m|^2>}_{I_M[l]} + \underbrace{\frac{2}{P}\left[ -\sum_{i=1}^{P}\Gamma[l-i] + \sum_{m=0}^{\delta}\Gamma[m] \right] <|d_m|^2>}_{C_N[l]} \tag{S17}$$

This expression (S17) shows explicitly that $I_N[l]$ is given by the sum of the conventional MS intensity $I_M$ and a coupling term $C_N$ . If we consider the case $l = 1$, we can see that $C_N$ vanishes and that $I_N[l=1] \simeq I_M[l=1]$.

An expression for the signal matrix elements $S[l,m]$ can also be found by substituting the expression for $\mathbf{A_R}$ [Eq. (S5)] and $\mathbf{A_N}$ [Eq. (S6)] into Eq. (S12):

$$S[l,m] = u_l^{(1)} r_m + u_l^{(1)} \sum_{i=1}^{P} u_i^{(1)*} c_i d_m \tag{S18}$$

One can then derive the corresponding intensity $I_S[l]$ [Eq. (S11)]

$$I_S[l] = \underbrace{\left|u_l^{(1)}\right|^2 <|r_m|^2>}_{I_R[l]} + \underbrace{\left\langle 2Re\left\{ r_l^* \sum_{i=1}^{P} u_i^{(1)*} c_i \sum_m d_m \right\} + \left| u_l^{(1)} \sum_{i=1}^{P} u_i^{(1)*} c_i d_m \right|^2 \right\rangle}_{C_S[l]} \tag{S19}$$

with $I_R$ the recurrent scattering intensity and $C_S$ a coupling term due to the residual multiple scattering intensity in the signal subspace. If we make the approximation that $\left|u_l^{(1)}\right|^2 \sim P^{-1}$ [Eq. (S8)], $C_S$ can be considered constant over $l$.

To estimate the residual multiple scattering contribution $C_S$, one can use the fact that the sum of $I_R$ and $I_M$ should be equal to the total intensity $I = <|a_{lm}|^2>$

$$I[l] = I_R[l] + I_M[l] \tag{S20}$$

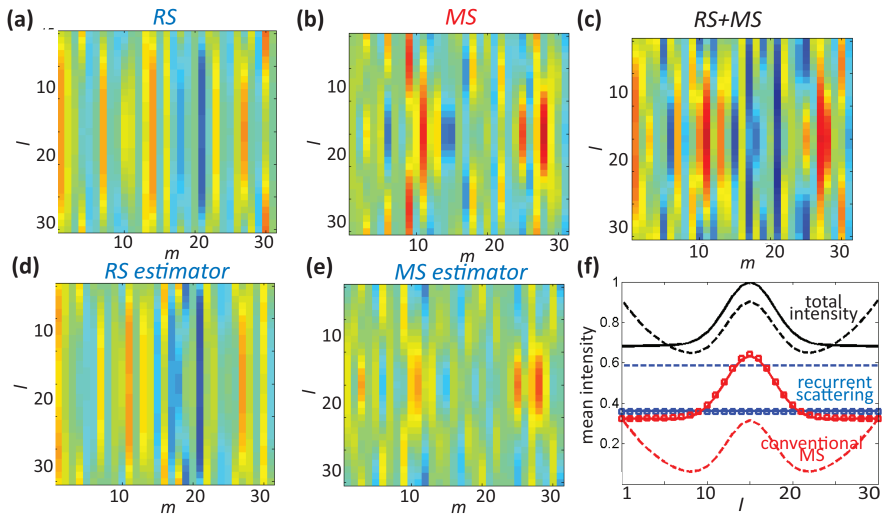


FIG. S2: Numerical validation of the RS/MS separation method. (a) Example of simulated RS matrix $\mathbf{A}'_\mathbf{R}$. (b) Example of simulated MS matrix $\mathbf{A}'_\mathbf{M}$. (c) Corresponding matrix $\mathbf{A}' = \mathbf{A}'_\mathbf{R} + \mathbf{A}'_\mathbf{M}$. (d) Estimated RS matrix $\hat{\mathbf{A}}'_\mathbf{R}$. (e) Estimated MS matrix $\hat{\mathbf{A}}'_\mathbf{M}$. (f) Intensity profiles (continuous line): $I_R$(blue), $I_M$ (red) and $I$ (black) - Estimated intensity profiles before correction (dashed lines): $I_S$ (blue), $I_N$ (red) and $I_N + I_S$ (black). Estimated intensity profiles after correction (square symbols): $\hat{I}_R$ (blue) and $\hat{I}_N$ (red).

Using Eqs. (S17)-(S19), we obtain

$$C_S + C_N[l] = I_S[l] + I_N[l] - I[l] \tag{S21}$$

Considering the last equation when $l = 1$ and recalling that $C_N[l = 1] \simeq 0$ allows one to calculate the coefficient $C_S$

$$C_S \simeq I_S[l = 1] + I_N[l = 1] - I[l = 1] \tag{S22}$$

Once $C_S$ is known, one can deduce estimators for the RS intensity and the conventional MS intensity:

$$\hat{I}_R[l] = I_S[l] - C_S \tag{S23}$$
$$\hat{I}_M[l] = I[l] - I_S[l] - C_S \tag{S24}$$

This operation is illustrated in Fig. S1(f). We check that $\hat{I}_M$ displays a profile typical of multiple scattering: a coherent backscattering peak on top of a flat incoherent background with an enhancement factor close to 2.

Estimators for the matrices $\mathbf{A_R}$ and $\mathbf{A_M}$ can be obtained by renormalizing $\mathbf{S}$ and $\mathbf{N}$ such that $\hat{I}_R[l] =< |\hat{A}_R[l,m]|^2 >$ and $\hat{I}_M[l] =< |\hat{A}_M[l,m]|^2 >$. This renormalization yields

$$\hat{\mathbf{A}}_\mathbf{R} = \alpha \mathbf{S},\ \hat{\mathbf{A}}_\mathbf{M} = \mathbf{A} - \alpha \mathbf{S}, \quad \text{with } \alpha = \sqrt{1 - C_S/I_S[1]} \tag{S25}$$

This operation is illustrated in Fig. S1. $\hat{\mathbf{A}}_\mathbf{R}$ and $\hat{\mathbf{A}}_\mathbf{M}$ shown in Figs. S1(g)-(h) are obtained following the renormalization of $\mathbf{S}$ and $\mathbf{N}$ [Figs. S1(d)-(e)].

### Back-rotation of data

The last step is the reverse of the first one. From $\hat{\mathbf{A}}_\mathbf{R}$ and $\hat{\mathbf{A}}_\mathbf{M}$, two estimators of the matrices $\mathbf{K_R}$ and $\mathbf{K_M}$, of dimension $(2M - 1) \times (2M - 1)$, are built [see Fig. S1(i)-(j)] with a change of coordinates, back to the original system:

- if $(s - r)/2$ is an integer,

then, $\hat{K}_{R,M}[s,r] = \hat{A}^{(1)}_{R,M}[(s - r)/2 + M, (s + r)/2]$

- if $(s - r)/2$ is not an integer,

then, $\hat{K}_{R,M}[s,r] = \hat{A}^{(2)}_{R,M}[(s - r - 1)/2 + M, (s + r - 1)/2]$

$\hat{\mathbf{K}}_\mathbf{R}$ and $\hat{\mathbf{K}}_\mathbf{M}$ are estimators of the RS contribution and of the conventional MS contribution, respectively.

### Numerical validation of the RS/MS separation method

In order to validate our approach, a numerical test has been performed by generating random matrices with the same statistical properties as the experimental antidiagonal matrices.

The RS antidiagonal matrix $\mathbf{A_R}$ has been simulated numerically as follows. The procedure first consists in generating numerically a line vector $\mathbf{R}$ whose elements are circularly symmetric complex Gaussian random variables with zero mean. Then a matrix $\mathbf{A}'_\mathbf{R}$ is built by multiplying the column vector $\mathbf{U}^{(1)}$ [Eq. (S8)] with the random line vector $\mathbf{R}$ [Eq. (S5)]. One can show that the matrix $\mathbf{A}'_\mathbf{R} = \mathbf{U}^{(1)}\mathbf{R}$ exhibits the same correlation properties as the experimental RS antidiagonal matrix $\mathbf{A_R}$. The parameters that appear in the expression of vector $\mathbf{U}^{(1)}$ [Eq. (S8)] are chosen to be the same as in the experiment: $a = 182$ mm, $p = 0.5$ mm, $f = 1.2$ MHz. An example of numerical matrix $\mathbf{A}'_\mathbf{R}$ thus obtained is shown in Fig. S2(a).

As for the conventional MS contribution, the correlation coefficient $\Gamma_l$ is first assumed to follow a Gaussian dependence $\Gamma_l = \exp(-l^2/\delta^2)$. We will consider a correlation length of 4 array pitches ($\delta = 4$), a typical value in our experiment. From this correlation coefficient, one can build a covariance matrix $\mathbf{J}$ whose coefficients are given by $J_{ij} = \Gamma_{i-j}$. The next step consists in generating numerically a random column

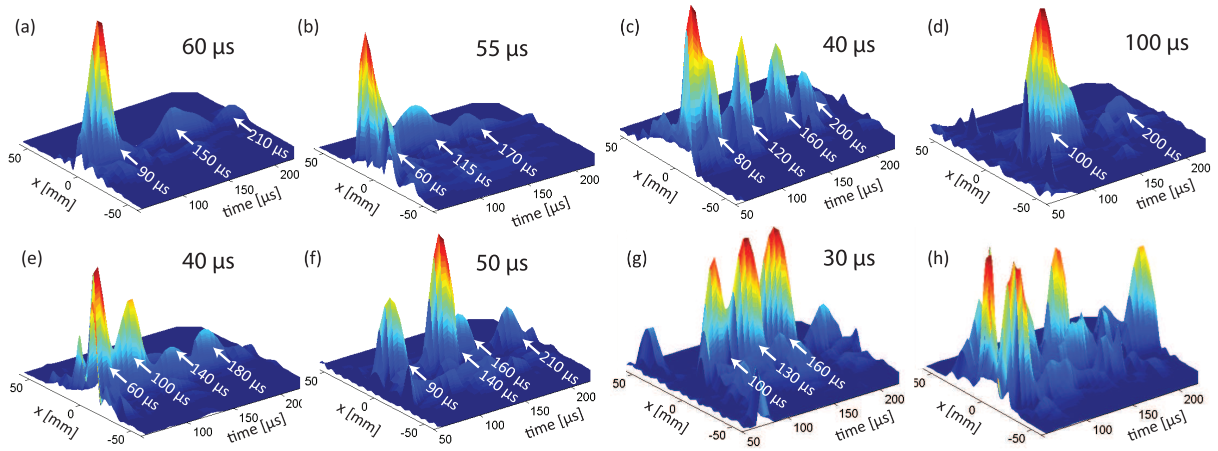


FIG. S3: Backpropagation of the first singular vector versus time at the sample surface for eight realizations of disorder at frequency $f = 1.2$ MHz. $x$ represents the coordinate along the surface.

vector $\mathbf{R}'$ whose elements are circularly symmetric complex Gaussian random variables with zero mean. Then, a correlated random vector $\mathbf{B}$ is built from $\mathbf{R}'$, such that

$$\mathbf{B} = \mathbf{J}^{\mathbf{1/2}}\mathbf{R}' \quad \text{(S26)}$$

One can show that the entries of $\mathbf{B}$ exhibit the correlation coefficient $\Gamma_l$. The antidiagonals should also exhibit the features of spatial reciprocity and of coherent backscattering in the MS regime. To that aim, a new column vector $\mathbf{C} = [c_l]$ is built by summing $\mathbf{B} = [b_l]$ and its flipped counterpart $\mathbf{B}' = [b_{P-l}]$ such that:

$$c_l = b_l + b_{P-l} \quad \text{(S27)}$$

This vector $\mathbf{C}$ is finally multiplied by a random line vector $\mathbf{D}$ to yield a matrix $\mathbf{A}'_\mathbf{M} = \mathbf{C} \times \mathbf{D}$ [Eq. (S6)]. This matrix thus generated displays the same properties as the experimental MS matrix $\mathbf{A_M}$. An example of numerical matrix $\mathbf{A}'_\mathbf{M}$ is shown in Fig. S2(b). As expected, it displays medium-range correlations along its columns. It also exhibits the feature of spatial reciprocity since each line of its upper part is identical to a line of its lower part: $A'_M[l,m] = A'_M[P-l,m]$. The corresponding intensity profile $I_M[l]$ has been calculated by averaging $|A'_M[l,m]|^2$ over $m$ and over 1000 different realizations. $I_M$ is displayed in Fig. S2(f) and exhibits a coherent backscattering cone whose line shape is governed by the correlation coefficient $\Gamma_l$.

Once the matrices $\mathbf{A}'_\mathbf{R}$ and $\mathbf{A}'_\mathbf{M}$ are obtained, one can build the matrix $\mathbf{A}'$ [Fig. S2(c)] as the sum of the RS and MS contributions [Eq. (S4)]. The corresponding intensity profile $I[l] =< |A'_R[l,m]|^2 + |A'_M[l,m]|^2 >$ is shown in Fig. S2(f). It displays a coherent backscattering peak with a linewidth and an enhancement factor similar to experimental results [see Fig. S1(f)].

The previously described RS/MS separation method has been tested on randomly generated antidiagonal matrices $\mathbf{A}$. To that aim, we have projected the matrix $\mathbf{A}'$ over the RS eigenvector $\mathbf{U}^{(\mathbf{1})}$ which yields the signal subspace $\mathbf{S} = \mathbf{U}^{(\mathbf{1})}\mathbf{U}^{(\mathbf{1})\dagger}\mathbf{A}'$ and the noise subspace $\mathbf{N} = \mathbf{A}' - \mathbf{S}$. The corresponding intensity profiles are shown in dashed lines in Fig. S2(f). As for experimental data, the noise subspace does not provide an intensity profile typical of multiple scattering (flat incoherent background). However, once the correction given by Eq. (S23) is applied [square symbols in Fig. S2(f)], the mean intensity profiles $I_R$ and $I_M$ are nicely recovered.

As for the estimators of the RS and MS matrices $\hat{\mathbf{A}}'_\mathbf{R}$ and $\hat{\mathbf{A}}'_\mathbf{M}$, the agreement is not as good as for the intensity profiles but still acceptable. The RS and MS estimators shown in Figs. S2(d)-(e) are compared to the RS and MS matrices $\mathbf{A}'_\mathbf{R}$ and $\mathbf{A}'_\mathbf{M}$ [Figs. S2(a)-(b)]. The averaged degree of similarity between those matrices reaches values of 90% and 80% for RS and MS, respectively.

This numerical test validates our method under the conditions of our experiment. One has to remember that two main conditions have to be fulfilled for the RS/MS separation method to be successful: $2a/k_w >> p^2\delta^2$ and $P >> \delta$.

## RECURRENT SCATTERING HOT SPOTS

In the Letter, the singular value decomposition of the matrix $\mathbf{K}$ has been investigated. A one-to-one correspondence has been demonstrated between the highest singular values and predominant recurrent scattering paths around 1.2 MHz. The first singular vector $\mathbf{V_1}$ back-focuses on the same particular location at regular time intervals (every 40 $\mu$s for the example shown in the Letter). Our hypothesis is that this hot spot corresponds to the entry/exit point of a RS path at the surface of the sample. The occurrence of the same hot spot periodically in time seems to indicate that it corresponds to successive round trips along the same RS path.

The goal of this supplementary material is to demonstrate that this result is not specific to the configuration of disorder considered in the Letter. To that aim, the backpropagation

of $\mathbf{V_1}$ is shown in Fig. S3 for eight other configurations of disorder. Except in Fig. S3(h), $\mathbf{V_1}$ back-focuses on particular locations at regular time intervals [Figs. S3(a)-(f)]. These time intervals depend on the realization of disorder, with values ranging from 30 $\mu$s [Fig. S3(g)] to 100 $\mu$s [Fig. S3(d)]. The variation of this time interval according the realization of disorder strongly suggests that these hot spots are not due to specular reflections from the front and back sample boundaries, since then the intervals would be the same whatever the configuration of disorder. Note that in Fig. S3(f), $\mathbf{V_1}$ back-focuses onto two different locations: $x = 12.5$ mm at times $t = 90$ and 160 $\mu$s, and $x = 9$ mm at times $t = 140$ and 210 $\mu$s. The emergence of these two hot spots separated by the same interval of time could indicate that they share parts of the same recurrent scattering path.


[S1] A. Aubry and A. Derode, Phys. Rev. Lett. **102**, 084301 (2009).

[S2] A. Aubry and A. Derode, J. Appl. Phys. **106**, 044903 (2009).

[S3] A. Aubry and A. Derode, J. Acoust. Soc. Am. **129**, 225 (2011).

[S4] I. Freund, M. Rosenbluh, and S. Feng, Phys. Rev. Lett. **61**, 2328 (1988).

[S5] S. Feng, C. Kane, P. A. Lee, and A. D. Stone, Phys. Rev. Lett. **61**, 834 (1988).

[S6] I. Freund, M. Rosenbluh, and R. Berkovits, Phys. Rev. B **39**, 12403 (1989).

[S7] E. Akkermans and G. Montambaux, Mesoscopic Physics of Electrons and Photons (Cambridge University Press, London, 2006).
